# Supplementary material for: LEAF: Do Agent-as-Policy Robots Notice and Fix Their Own Failures?
Source: arXiv:2611.36670 source file (2026-11-26)
Supplement: Supplementary file 1 [file appendix_behaviour.tex]

\begin{table}[H]
\centering
\footnotesize
\setlength{\tabcolsep}{2.6pt}
\caption{\textbf{What agents do around a failure}, single-cause tasks, in \%. Hold: first gripper closure holds the object (84 grasping instances). Slip / Trap: instances with an in-attempt repair of the agent's own slip / of a sprung trap (102). Break: attempts breaking a completed step (13 tasks that log subgoals); Succ.\ b / i: success with a broken / intact step; Restore: broken attempts with every lost step restored. Right: correct success claims, nearly invisible failures excluded.}
\label{tab:behaviour}
\begin{tabular}{@{}lccccccc@{}}
\toprule
 & \multicolumn{3}{c}{Execution} & \multicolumn{3}{c}{Completed steps} & Claims \\
\cmidrule(lr){2-4}\cmidrule(lr){5-7}\cmidrule(l){8-8}
Model & Hold & Slip & Trap & Break & Succ.\ b / i & Restore & Right \\
\midrule
GPT-6 Astra & 40 & 22 & 25 & 52 & 28 / 59 & 25 & 96 \\
Opus~5.5 & 68 & 11 & 25 & 36 & 21 / 50 & 32 & 91 \\
Sonnet~5.5 & 30 & 15 & 13 & 53 & \phantom{0}2 / 31 & 11 & 76 \\
DeepSeek & 11 & \phantom{0}5 & \phantom{0}3 & 25 & \phantom{0}3 / \phantom{0}2 & 10 & 59 \\
\bottomrule
\end{tabular}
\end{table}
