# Supplementary material for: LEAF: Do Agent-as-Policy Robots Notice and Fix Their Own Failures?
Source: arXiv:2611.36670 source file (2026-11-26)
Supplement: Supplementary file 2 [file appendix_decisive.tex]

\begin{table}[H]
\centering
\footnotesize
\setlength{\tabcolsep}{3pt}
\caption{\textbf{Retries do not change the choice that decides the outcome.} Attempts in the main runs against fresh agents told the cause, by model, in \% of attempts. GPT was not run with the cause stated on clear cover and soft-box stacking.}
\label{tab:decisive}
\begin{tabular}{@{}>{\raggedright\arraybackslash}p{0.15\linewidth}>{\raggedright\arraybackslash}p{0.19\linewidth}>{\raggedright\arraybackslash}p{0.30\linewidth}>{\raggedright\arraybackslash}p{0.27\linewidth}@{}}
\toprule
Task & Decisive choice & Retries, told only success or failure & Told the cause \\
\midrule
Clear cover & Remove the lid & Removed in 0\% of attempts, four models & Opus removes it and succeeds in 75\% \\
Card shelf & Do not push the weighted end & After pushing it and failing, GPT and Opus push it again in 91\% & Opus and GPT push the light end and succeed in 100\% \\
Soft-box stacking & Do not load the soft box & After a collapse, the next attempt collapses again in 88\% & Opus: 0\% collapse, 100\% succeed \\
Fit container & Pick the right box & Right box: GPT 50\%, Opus 22\%, Sonnet 22\%, DeepSeek 0\% & Opus succeeds in 100\% (also with the error alone); GPT picks it in 100\% but still rests it on the rim in 67\% \\
\bottomrule
\end{tabular}
\end{table}
