# Supplementary material for: LEAF: Do Agent-as-Policy Robots Notice and Fix Their Own Failures?
Source: arXiv:2611.36670 source file (2026-11-26)
Supplement: Supplementary file 3 [file appendix_history_grid.tex]

\begin{figure}[H]
  \centering
  \includegraphics[width=\linewidth]{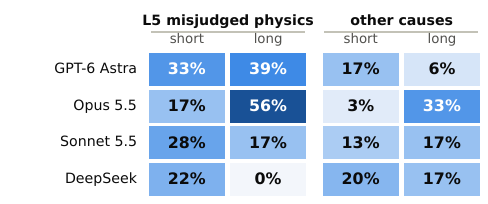}
  \caption{\textbf{Where history helps.} Share of the 84 paired single-cause instances solved within three attempts with history but not by memory-free retries, by failure cause and task length (long: the twelve long-horizon single-cause tasks).}
  \label{fig:history-split}
\end{figure}
